# Supplementary material for: Pulsed Rabi oscillations in quantum two-level systems: beyond the Area Theorem
Source: arXiv:1708.05444 ancillary file (2017-11-03)
Supplement: Supplementary file 1 [file Supplemental_material.pdf]

# Supplementary material—Pulsed Rabi oscillations in quantum two-level systems: beyond the Area Theorem

Kevin A. Fischer,[1,*] Lukas Hanschke,[2] Malte Kremser,[2] Jonathan J. Finley,[2] Kai Müller,[2] and Jelena Vučković[1]
[1]*E. L. Ginzton Laboratory, Stanford University, Stanford CA 94305, USA*
[2]*Walter Schottky Institut, Technische Universität München, 85748 Garching bei München, Germany*
(Dated: August 23, 2017)

## I. SAMPLE DESIGN

The sample investigated is grown by molecular beam epitaxy (MBE). It consists of a layer of InGaAs quantum dots with low areal density ($< 1\,\mu\text{m}^{-2}$), embedded within the intrinsic region of a Schottky photodiode formed from an n-doped layer below the quantum dots and a semi-transparent titanium gold front contact. The distance between the doped layer and the quantum dots is 35 nm, which enables control over the charge status of the dot [1]. A weak planar microcavity with an optical thickness of one wavelength ($\lambda$) is formed from a buried 18 pair GaAs/AlAs distributive Bragg reflector (DBR) and the semitransparent top contact, which enhances the in- and out-coupling of light.

The electric-field-dependent photoluminescence of the QD is presented in Fig. 1 and shows clear charge stability plateaus for the neutral exciton ($X^0$) as well as for the single electron to negative trion ($X^-$) transition. We measure the lifetime of the negative trion $X^-$ under resonant excitation to be 420ps.

## II. MEASUREMENT SETUP

All optical measurements were performed at 4.2 K in a liquid helium dipstick setup. For excitation and detection, a lens with a numerical aperture of $NA = 0.68$ was used. Cross-polarized measurements were performed using a polarizing beam splitter. To further enhance the extinction ratio, additional thin film linear polarizers were placed in the excitation/detection pathways and a single mode fiber was used to spatially filter the detection signal. Furthermore, a quarter-wave plate was placed between the beamsplitter and the microscope objective to correct for birefringence of the optics and sample itself [2].

Excitation pulses with a length $< 80$ ps were derived from a fs-pulsed titanium sapphire laser (Coherent Mira 900) through pulse shaping. For pulses $< 30$ ps, a 4f pulse shaper with a focal length of 1 m and an 1800 l/mm grating was used. For the 80 ps long pulses a spectrometer-like filter with a focal length of 1 m and an 1800 l/mm grating was used. Longer pulses were obtained through modulating a continuous wave laser. For the modulation a fiber coupled and EOM controlled lithium niobate Mach-Zehnder interferometer with a bandwidth of 10 GHz (Photline NIR-MX-LN-10) was used. Such modulators allow control of the output intensity through a DC bias and a radio frequency input. The radio frequency pulses were generated by a 3.35 GHz pulse-pattern generator (Agilent 81133A). To obtain a high extinction ratio, the temperature of the modulator was stabilized and precisely controlled (within 1 mK) using a Peltier element, thermistor, and TEC controller. This enabled a static extinction ratio $> 50$ dB.

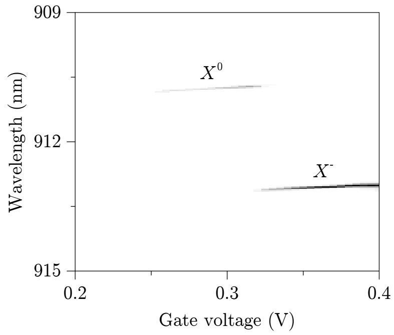


FIG. 1. Photoluminescence versus applied gate bias and wavelength showing the charge-stability region of the $X^-$ transition.

## III. SECOND-ORDER COHERENCE MEASUREMENTS

Second-order autocorrelation measurements were performed using a Hanbury Brown and Twiss (HBT) setup consisting of one beamsplitter and two single-photon avalanche diodes [3]. The detected photons were correlated with a TimeHarp200 time counting module. The integration times were between one and two hours.

The measured degree of second-order coherence $g^{(2)}[0]$ as a function of the pulse length is presented in Fig. 2a. At each data point, a pulse area of $\pi$ was used. This area was directly obtained for short pulses through measuring Rabi oscillations and extrapolated for longer pulses, based on the Area Theorem (eq. 1 in the main text). For short pulses an increase in $g^{(2)}[0]$ with decreasing pulse length is observed. This is a measurement artifact that results from the wavelength dependence of our cross-polarized suppression. When the pulses get shorter

* kevinf@stanford.edu

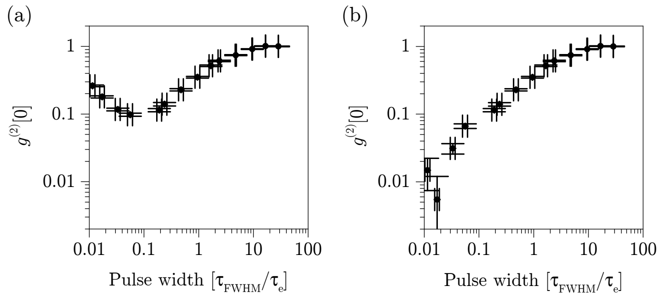


FIG. 2. Measured degree of second-order coherence $g^{(2)}[0]$ for emission from a two-level system under interaction with a $\pi$-pulse, i.e. $A(\infty) = \pi$. Data obtained when resonantly exciting a two-level system made up of excitonic states from a deterministically charged quantum dot. (a) Raw correlation data and (b) correlation data corrected for background.

in time, they become broader in energy and have spectral components further away from the QD transition. Since the cross-polarized suppression is optimized at the QD frequency, these components start to leak into the detection channel. To correct for this artifact, for each pulse length we directly measured the ratio of photons emitted from the QD to photons resulting from imperfect suppression by electrically tuning the quantum dot out of resonance. Taking this ratio into account in the calculation of $g^{(2)}[0]$ results in the data presented in Fig. 2b (and in Fig. 1c of the main text). The x-error results from the $\sqrt{N}$ error in the photocount distribution while the y-error results from experimental inaccuracies in determining the pulse length.

As discussed in the main text, the data produces overall good agreement with the simulations. Small deviations are most likely to result from the experimental error in determining the pulse area of $\pi$ and inaccuracies in the pulse shape, as well as drifts and fluctuations in power and suppression over the duration of the measurements. As recently experimentally shown, small power fluctuations can result in significant changes in the second-order coherence [3, 4]. Additionally, dephasing mechanisms [5] may contribute to a slightly increased $g^{(2)}[0]$, because they may re-excite the system more quickly than the laser pulse would alone. These mechanisms are also roughly linear with the pulse width, like coherent re-excitation, because the limiting rate is still the emission of a photon from the system.

[1] R. J. Warburton, C. Schaflein, D. Haft, F. Bickel, *et al.*, *Optical emission from a charge-tunable quantum ring,* Nature **405**, 926 (2000).

[2] A. V. Kuhlmann, J. Houel, D. Brunner, A. Ludwig, D. Reuter, A. D. Wieck, and R. J. Warburton, *A dark-field microscope for background-free detection of resonance fluorescence from single semiconductor quantum dots operating in a set-and-forget mode,* Rev. Sci. Instrum. **84**, 073905 (2013).

[3] K. A. Fischer, K. Müller, K. G. Lagoudakis, and J. Vučković, *Dynamical modeling of pulsed two-photon interference,* New J. Phys. **18**, 113053 (2016).

[4] K. A. Fischer, L. Hanschke, J. Wierzbowski, T. Simmet, C. Dory, J. J. Finley, J. Vučković, and K. Müller, *Signatures of two-photon pulses from a quantum two-level system,* Nat. Phys. (2017).

[5] A. C. Dada, T. S. Santana, R. N. Malein, A. Koutroumanis, Y. Ma, J. M. Zajac, J. Y. Lim, J. D. Song, and B. D. Gerardot, *Indistinguishable single photons with flexible electronic triggering,* Optica **3**, 493 (2016).
